# Supplementary material for: Magnon gap excitations in van der Waals antiferromagnet MnPSe$_3$
Source: arXiv:2309.06866 source file (2023-09-13)
Supplement: Supplementary file 1 [file MnPSe3_Magnon_SM.pdf]

# Supplemental Material for "Magnon gap excitations in van der Waals antiferromagnet $MnPSe_3$"

Dipankar Jana,[1,*] D. Vaclavkova,[1] I. Mohelsky,[1] P. Kapuscinski,[1,2] C. W. Cho,[1] I. Breslavetz,[1] M. Białek,[3,4] J.-Ph. Ansermet,[4] B. A. Piot,[1] M. Orlita,[1,5] C. Faugeras,[1] and M. Potemski[1,3,†]

[1] *Laboratoire National des Champs Magnétiques Intenses, LNCMI-EMFL, CNRS UPR3228, Univ. Grenoble Alpes, Univ. Toulouse, Univ. Toulouse 3, INSA-T, Grenoble and Toulouse, France*
[2] *Institute of Experimental Physics, Faculty of Physics, University of Warsaw, ul. Pasteura 5, PL-02-093 Warsaw, Poland*
[3] *CENTERA Labs, Institute of High Pressure Physics, PAS, 01-142 Warsaw, Poland*
[4] *Institute of Physics, Ecole Polytechnique Fédérale de Lausanne (EPFL), 1015 Lausanne, Switzerland*
[5] *Institute of Physics, Charles University, Ke Karlovu 5, Prague, 121 16, Czech Republic*

## I. THz MONOCHROMATIC TRANSMISSION MEASUREMENTS

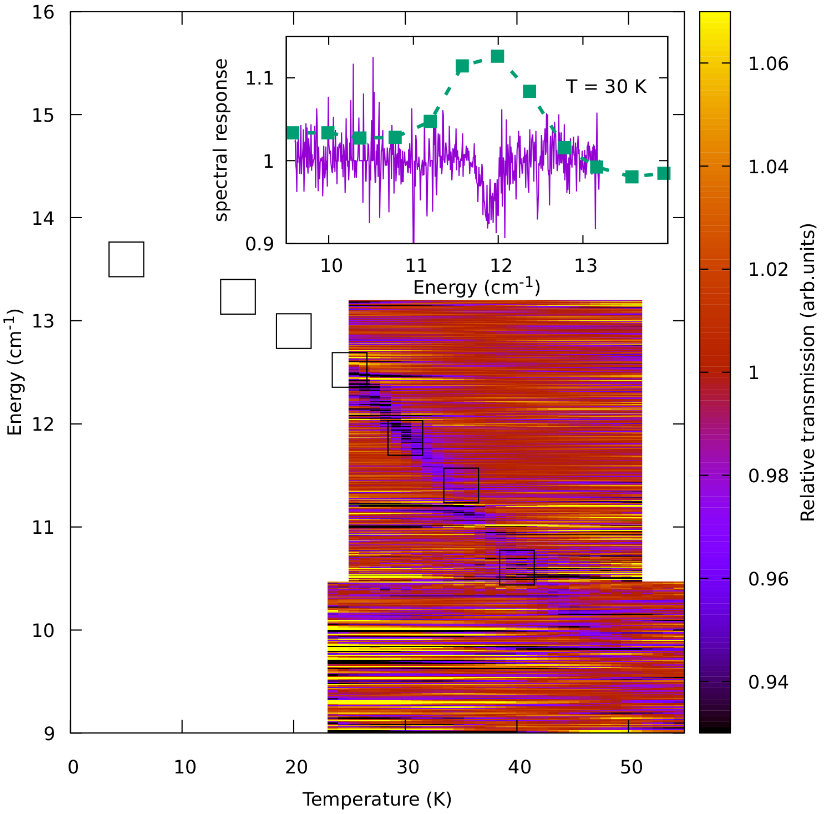


FIG. S1. False color map of normalised THz transmission spectra of $MnPSe_3$, at $B = 0$ $T$, as a function of temperature in the spectral range from 9 to 13 $cm^{-1}$. A bulk sample of $MnPSe_3$ was placed on an aperture in a closed-cycle cryostat with optical windows. We used a monochromatic spectrometer based on frequency extenders to a vector network analyzer. See Ref. [S1] for the extended information on the experimental set-up applied. The energy positions of the upper magnon mode determined from Raman scattering measurements (see Fig. 1b. of the main text) are shown with open rectangles. An example of a (relative) transmission spectrum, measured at 30 K, is shown in the inset and compared to the corresponding Raman scattering signal shown with the dashed line. Linewidth determined using monochromatic THz spectroscopy data is about 0.1 $cm^{-1}$.

* dipankar.jana@lncmi.cnrs.fr
† marek.potemski@lncmi.cnrs.fr

## II. RAMAN SCATTERING SPECTRA OF $MnPSe_3$, MEASURED AS A FUNCTION OF THE MAGNETIC FIELD APPLIED IN NEARLY OUT-OF-PLANE CONFIGURATION

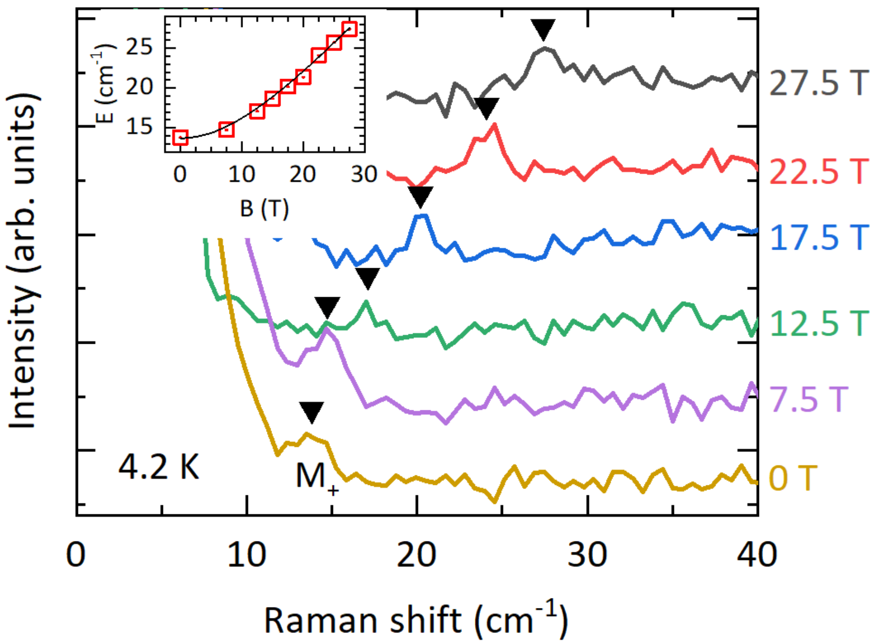


FIG. S2. Magneto-Raman scattering spectra of $MnPSe_3$, measured at 4.2 K, at several values of the magnetic field $B$. The $B$-field is applied at an angle of 20° with respect to the normal to the layers' plane. Only $M_+$ resonance could be traced in this experiment; the response due to the lower $M_-$ magnon gap is hidden by the insufficiently rejected stray laser light. The dependence of the energy of the $M_+$ resonance upon the applied magnetic field is shown in the inset. As discussed in the main text, it follows the $w_{M+}(B) = \sqrt{(w_{M+})^2 + (g\mu_B B\cos(20°))^2}$ dependence as shwon by the solid line.

## III. RAMAN SCATTERING SPECTRA OF $MnPSe_3$, MEASURED AS A FUNCTION OF THE IN-PLANE MAGNETIC FIELD (UP TO 30 T), IN A WIDE SPECTRAL RANGE.

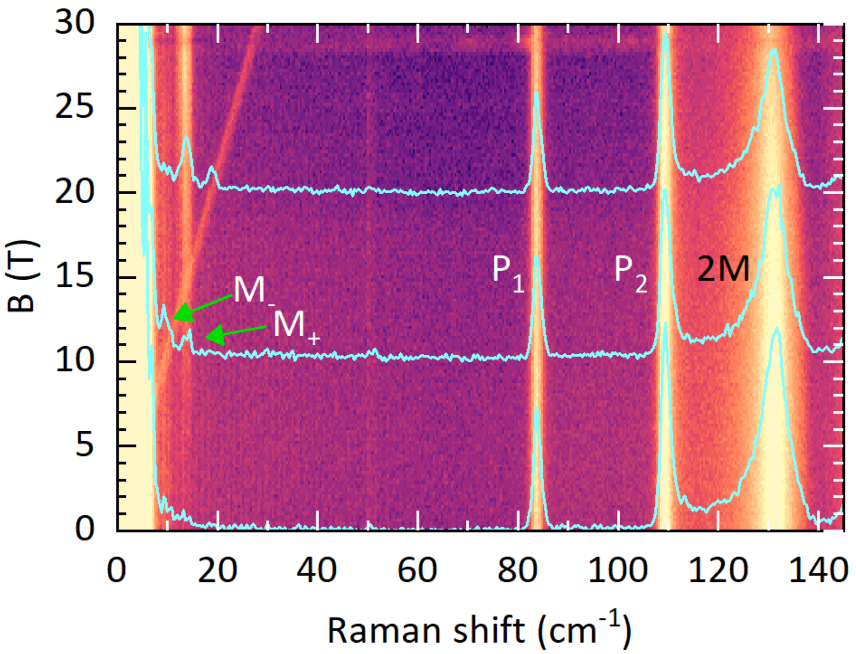


FIG. S3. False color map of Raman scattering spectra of $MnPSe_3$, measured at 4.2 K, as a function of the magnetic field applied in layers' a-b plane. A few representative spectra, measured at a magnetic field strength of 0 T, 10 T, and 20 T are also plotted. $M_+$ and $M_-$ resonances correspond to the upper and lower magnon gap excitation which shows a crossover at around 14 T. $P_1$, $P_2$ correspond to phonon modes while 2M is due to two magnon excitation[S2].

## IV. SIMULATION FOR THE IN-PLANE MAGNETIC FIELD DEPENDENCE OF MAGNON GAP EXCITATIONS IN A BIAXIAL $MnPSe_3$ ANTIFERROMAGNET

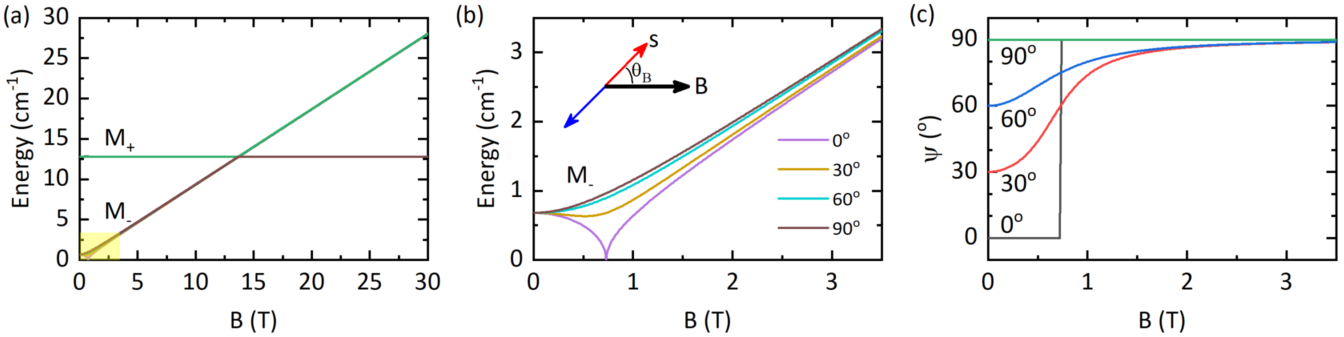


FIG. S4. (a) Simulated in-plane magnetic field dependence of low $M_-$ and high $M_+$ energy magnon modes, in a broad range of magnetic fields, up to 30 T, for different $\theta_B$ angle between the direction of the applied magnetic field and the axis along which the spins are initially (at $B = 0$) aligned. (b) The dependence of $M_-$ mode in the low field region as highlighted in Fig S4a for different $\theta_B$, and (c) Upon the application of the in-plane magnetic field, the orientation of spins with respect to the direction of the magnetic field changes. As illustrated, the angle $\Psi_B$ between the $B$ direction and the axis of spin alignments evolves differently for different initial $\theta_B$, angles.

[S1] M. Białek, T. Ito, H. Rønnow, and J.-P. Ansermet, Terahertz-optical properties of a bismuth ferrite single crystal, Phys. Rev. B **99**, 064429 (2019).

[S2] T. T. Mai, K. F. Garrity, A. McCreary, J. Argo, J. R. Simpson, V. Doan-Nguyen, R. V. Aguilar, and A. R. H. Walker, Magnon-phonon hybridization in 2D antiferromagnet $MnPSe_3$, Sci. Adv. **7**, eabj3106 (2021).
